# Supplementary material for: Uncertainty-aware Human Mobility Modeling and Anomaly Detection
Source: arXiv:2410.01281 source file (2025-05-05)
Supplement: Supplementary file 1 [file tab_AD_score_func_additional.tex]

\begin{wraptable}{r}{0.55\linewidth} % 'r' for right, 'l' for left, width of the figure
    \vspace{-0.15in}
    \caption{Results of additional different anomaly scoring functions}
    \vspace{-0.1in}
    \centering
    
    \setlength\tabcolsep{2 pt}
    \resizebox{1\linewidth}{!}{
    \begin{tabular}{c|cc|cc|cc}
    \toprule
        \multirow{2}{*}{Function} & \multicolumn{2}{|c|}{\trial (small)} & \multicolumn{2}{|c|}{\NUMOSIM(small)} & \multicolumn{2}{|c}{\NUMOSIM(20K)}  \\
        \cline{2-7}
          & AUROC & AUPR & AUROC & AUPR & AUROC & AUPR \\
         \midrule
         $\Delta_f$  & 0.666 & 0.200 & 0.553 & 0.062 & 0.556 & 0.003\\
         \cline{1-7}
         $\text{pth}(\Delta_f)$  & \underline{0.789} & \underline{0.295} & \textbf{0.694} & \underline{0.143} & \underline{0.699} & \underline{0.031} \\
         \cline{1-7}
         $\text{pth}\left(\frac{\Delta_f}{1+\alpha_f+\beta_f}\right)$ & \textbf{0.795} & \underline{0.329} & \textbf{0.694} & \textbf{0.147} & \textbf{0.700} & \textbf{0.034} \\
    \bottomrule
    \end{tabular}
    }
    \label{tab:ablation_AD_score}
    \vspace{-0.1in}
\end{wraptable}
